# Supplementary material for: Global Optimality Guarantees For Policy Gradient Methods
Source: arXiv:1906.01786 source file (2022-06-20)
Supplement: Supplementary file 1 [file appendix_rates.tex]

%!TEX root = policy_grad_optimality.tex
\section{Convergence proofs for first order methods.}
\label{app:proof_of_convergence_rates}

To start, let us define some standard notions from first order optimization. For a convex set $\Xc \subset \mathbb{R}^d$, we say a function $f:\Xc \to \mathbb{R}$ is $k$-Lipshitz if $\norm{f(x) - f(y)}_2 \leq k \norm{x - y}_2$ for every $x,y \in \Xc$. We say a function is $L$-smooth if $f$ is differentiable throughout $\Xc$ and $\nabla f$ is $L$-Lipschitz. A consequence of smoothness that will be useful throughout our proofs is often called the \textit{descent lemma}. It implies a quadratic upper bound on function values. The proof follows by Taylor expansion and the mean-value theorem \citep{bertsekas1997nonlinear}.
\begin{lem}[Descent Lemma] \label{lemma:smoothness}
	If the function $f:\D\to \mathbb{R}$ is $L$-smooth over a set $\X \subseteq \D$, then for any $(x,y) \in \X$:
	\[
	f(y) \leq f(x) + \langle \nabla f(x), y-x \rangle + \frac{L}{2} \norm{y-x}^2_2.
	\]
\end{lem}

The following interpretation of projected gradient updates will be very useful for our proof. Recall the notation for orthogonal projection: ${\rm Proj}_{\X} (x) = \argmin_{y \in \X} \, \norm{y - x}^2_2$. The projected gradient descent iteration can be equivalently written as 
\begin{align}\label{eq:quad_approx_appendix}
x_{t+1} = {\rm Proj}_\X \left( x_t - \alpha_t \nabla f(x_t) \right) =  \argmin_{x \in \X} \left[ f(x_t) + \langle \nabla f(x_t), x-x_t \rangle + \frac{1}{2\alpha_t} \norm{x-x_t}^2_2 \right].
\end{align} 
giving a ``proximal'' interpretation of projection as minimizing a local quadratic approximation. See \cite{beck2017first} for a simple proof.

\subsection{Asymptotic convergence to stationary points: proof of Lemma \ref{lem: pgd reaches global optimum}}
For convenience, we first restate the claim. 
\convergencetostationary*
\begin{proof}
	%Part 1 follows from \cite[Proposition 3.6.3]{bertsekas1997nonlinear} or \cite[Theorem 10.15]{beck2017first}.  
	Part 1 follows from the simple proofs in \citep{beck2002convergence, beck2017first}.
	We show the claim in part 2. Throughout, let $\| x\|$ denotes the Euclidean norm of a vector $x$ and $\|A\|= \max_{\|x\|\leq 2} \| Ax\|$ be induced operator norm of a matrix $A$.  Note that the sub-level set $S := \{x \in \Xc : f(x) \leq f(x_0) \}$ is compact (continuity of $f(\cdot)$ implies its closed and we assume it to be bounded). Also, for a sufficiently small $\epsilon$, $f(\cdot)$ is twice continuously differentiable over the compact set,
	\[
	S_{\epsilon} := \{ x +y:   x\in  S_1, \| y\| \leq \epsilon  \}. 
	\]
	which follows by our assumption that $f(\cdot)$ is twice continuously differentiable on an open set containing $S$. We denote $G = \max_{x\in S} \| \nabla f(x) \| $ and $L = \max_{x \in S_{\epsilon}} \| \nabla^2 f(x) \|$. Note that $G$ and $L$ are finite since $\|\nabla f\|$ and $\|\nabla^2 f\|$ are continuous  over the compact sets $S$ and $S_{\epsilon}$. Fix the step-size $\alpha= \min\{\epsilon / G, 1/L \}$. For any $x\in S_1$, define $x^{+} = {\rm Proj}_\X \left( x - \alpha \nabla f(x) \right)$. For this choice of step-size,  $x^+ \in S_{\epsilon}$ since
	\[
	\| x^{+} - x\|_2  = \|  {\rm Proj}_\X \left( x - \alpha \nabla f(x) \right) - {\rm Proj}_\X(x)  \| \leq \| \alpha \nabla f(x)\| \leq \alpha G \leq \epsilon,
	\]
	which follows as projection operators are non-expansive. The optimality conditions for projection onto a convex set yield the standard property that $\hat{x} = {\rm Proj}_\X \left( x\right)$ if and only if $\langle \hat{x}-x, y-\hat{x} \rangle \geq 0 $ for all $y\in \Xc$. Using this and some algebra, we get 
	\begin{align*}
	\langle x - \alpha \nabla f(x) - x^+, x - x^+ \rangle \leq 0 \,\, \implies \,\, \|x - x^+\|^2 - \alpha \langle \nabla f(x), x - x^+ \rangle  \leq 0.
	\end{align*}
	As $x^+ \in S_{\epsilon}$,
	\begin{flalign*}
    && f(x^+) &\leq  f(x) + \langle \nabla f(x)\, , \, x^+ - x \rangle  + \frac{L}{2} \| x^+ - x\|^2   && [\text{smoothness of} f(\cdot) \text{ over } S_\epsilon]\\
	&&   &\leq f(x) + \left( \frac{L}{2} - \frac{1}{\alpha} \right) \|x^+ - x\|^2 &&\\
	&&   &\leq f(x). &&  [\alpha  \leq 1/L]  
	\end{flalign*}
	Since the projected gradient update reduces cost, we know $x^+ \in S$. Repeating this argument inductively shows that $f(x_{k+1}) \leq f(x_k)$ and $x_k \in S$ for all $k$. 
	Since $\{x_k\}$ is contained in a compact set $S$, it has a convergent sub-sequence, $\{x_{k_i}\}$ with some limit $x_{\infty}$. We have ,
	\[ 
	\lim_{k\to \infty} f(x_k) = \lim_{i\to \infty} f(x_{k_i}) = f(x_\infty),
	\]
	where the first limit exists since $\{f(x_k) \}$ is monotone-decreasing and bounded below and the final inequality uses continuity of $f(\cdot)$. The proof to show that any limit point is a stationary point follows from \citep{beck2002convergence, beck2017first}. See also \citep[Figure 3.3.2]{bertsekas1997nonlinear}. We omit this for brevity.
\end{proof}

\subsection{Convergence rates under gradient dominance: Proof of Lemma \ref{lemma:second_order_convergence_rate}.}
We first restate the claim. 
\ratesgraddominance*

\begin{proof}[Proof of Lemma \ref{lemma:second_order_convergence_rate}]
Recall, by Definition \ref{def:gradient_dominance} that a function $f$ is defined to be $(c,\mu)$--\textit{gradient dominated} over $\Xc$ if there exists a constant $c>0$ and $\mu\geq 0$ such that
\[
f(x^*)  \geq f(x) + \min_{y\in \mathcal{X}} \, \left[ c\, \langle \nabla f(x),y-x\rangle + \frac{\mu}{2} \norm{y-x}^2_2 \right]  \,\, \quad \forall \, x\in \Xc. 
\]

\paragraph{Proof of Part (a):}
We assume $\mu=0$ in which case for any $x\in \Xc$, we have 
\begin{align}
		\label{eq:first_order_grad_dominance_app}
		\min_{y\in \mathcal{X}} \, \left[ c\, \langle \nabla f(x),y-x\rangle \right] \leq f(x^*) - f(x)
\end{align}
Therefore, for any $x \neq x^*$, we have $\min_{y \in \D} \, \langle \nabla f(x_t), y - x \rangle < 0$. Let $\{x_t\}$ be the iterates produced by projected gradient descent. At iterate $x_t$, let $\bar{y} = \argmin_{y \in \X} \, \langle \nabla f(x_t), y-x_t \rangle$ and denote $\delta_t = \min_{y \in \X} \langle \nabla f(x_t), y-x_t \rangle$. Note that $\delta_t \leq 0$ and $|\delta_t| \leq \|\nabla f(x_t)\| \|y-x_t\| \leq k R$ as $f$ is assumed to be $k$-Lipschitz. We take a constant stepsize, $\alpha_t = \alpha \leq \min\{ \frac{1}{k},\frac{1}{L}\}$. Then,

\begin{align}
f(x_{t+1}) - f(x_t) &\overset{(a)}{\leq} \min_{y \in \D} \, \left[ \langle \nabla f(x_t), y-x_t \rangle + \frac{1}{2\alpha} \norm{y-x_t}^2_2 \right] \nonumber \\
&\overset{(b)}{=} \min_{\beta \in [0,1]} \left[ \langle \nabla f(x_t), x_t + \beta(\bar{y}-x_t) - x_t \rangle + \frac{1}{2 \alpha} \norm{x_t + \beta(\bar{y}-x_t) - x_t}^2_2 \right] \nonumber \\
&= \min_{\beta \in [0,1]} \, \left[ \beta \langle \nabla f(x_t), (\bar{y}-x_t) \rangle + \frac{\beta^2}{2\alpha} \norm{\bar{y}-x_t}^2_2 \right] \nonumber \\
&\leq \min_{\beta \in [0,1]} \, \left[ \beta \delta_t + \frac{\beta^2 R^2}{2\alpha} \right] = \frac{-\alpha \delta_t^2}{2R^2} \label{eq:proj_rates1}
\end{align}
where the minimizer $\beta^*=-\delta_t\alpha / R^2 \leq k \alpha / R \leq 1$ as $\alpha \leq \min\{\frac{1}{k}, \frac{1}{L} \}$ (we assume $R>1$ without loss of generality as we can take any upper bound while minimizing in \eqref{eq:proj_rates1}).
Here (a) follows by using the equivalence shown in \eqref{eq:quad_approx_appendix} and the quadratic upper bound on the function values implied by the descent lemma. Equality (b) uses the fact that right hand side of (a) can be optimized by searching over the steepest descent direction $x_t \to y$. Using \eqref{eq:first_order_grad_dominance_app}, we get
\[
f(x_{t+1}) - f(x_t) \leq \frac{-\alpha}{2R^2 c^2} \left( f(x^*) - f(x_t) \right)^2
\]
Rearranging, we get our desired result
\begin{align*}
\min_{t \leq T}  \left( f(x_t) - f(x^*) \right)^2 \leq \frac{1}{T} \sum_{t=0}^{T-1} \left( f(x_t) - f(x^*) \right)^2 &\leq \frac{2R^2c^2}{\alpha T} \sum_{t=0}^{T-1} f(x_t) - f(x_{t+1}) \\
&\leq \frac{2R^2c^2}{\alpha T} \left( f(x_0) - f(x_T) \right) \\
&\leq \frac{2R^2c^2}{\alpha T} \left( f(x_0) - f(x^*) \right)
\end{align*}
Since also $f(x_T) \leq f(x_{T-1}) \leq \cdots f(x_1)$, we have
\[
f(x_T) - f(x^*) \leq \min_{t \leq T}  \left\{ f(x_t) - f(x^*) \right\} \leq \sqrt{\frac{2R^2c^2 \left( f(x_0) - f(x^*) \right)}{\alpha T}}.
\]

\paragraph{Proof of Part (b):} We refer readers to the proof in \cite{karimi2016linear}, which can be dated back to \cite{polyak1963gradient}.
\end{proof}

\subsection{Regularized finite state and action MDPs with nonlinear parameterization.}\label{app:softmax}
We continue the discussion of Example \ref{ex:vanishin_grads_softmax}. Given a feasible descent direction $D$, which by definition means  $\pi_{ \theta}+\alpha D \in \Pi$ is a feasible policy for sufficiently small $\alpha$, our goal is to verify that there exists $N$ solving the linear system $\left[ \frac{\partial \pi_{ \theta}}{\partial \theta} \right] N = D.$  For simplicity, imagine there is only a single state, so that a policy is described by the vector $(\pi_{\theta}(1),\cdots, \pi_{\theta}(k))$.
If there were multiple states, the same argument  could be repeated for each block of parameters corresponding to a distinct state. 	

Since we have effectively fixed a choice of $\theta_1=0$ in Example \ref{ex:vanishin_grads_softmax},  $\left[ \frac{\partial \pi_{ \theta}}{\partial \theta} \right] N = D$ is a system of $k$ equations with $k-1$ variables, denoted $N=(N_2, \cdots, N_k)$. We first temporarily ignore the first linear equality and show we can solve the remaining $k-1$ equations: 
$\frac{\partial \pi_{ \theta}(i) }{\partial \theta_2}N_2 + \cdots + \frac{\partial \pi_{ \theta}(i) }{\partial \theta_k}N_k = D_i$ for each $i\geq 2$. To see this, consider the  $(k-1)\times (k-1)$ submatrix of the Jacobian that comes from dropping the first row:
\[
\left[ \frac{\partial \pi_{ \theta}(i)}{\partial\theta_j } \right]_{i,j>2} = \begin{bmatrix}
	\pi_{ \theta}(2)(1-\pi_{ \theta}(2)) & -\pi_{ \theta}(2)\pi_{ \theta}(3) & \cdots & -\pi_{ \theta}(2)\pi_{ \theta}(k)\\
	-\pi_{ \theta}(2)\pi_{ \theta}(3)  & \pi_{ \theta}(3)(1-\pi_{ \theta}(3)) & \cdots & -\pi_{ \theta}(3)\pi_{ \theta}(k) \\   
	\vdots & \vdots & \vdots & \vdots \\
	-\pi_{ \theta}(2)\pi_{ \theta}(k) & -\pi_{ \theta}(3)\pi_{ \theta}(k) & \cdots & \pi_{ \theta}(k)(1-\pi_{ \theta}(k))
\end{bmatrix}.
\]
This matrix is diagonally dominant and therefore non-singular, implying a solution to these $k-1$ linear equations exist.

We now show that the first linear equation is redundant and follows from the other $k-1$. In particular, we have 
\[
\sum_{j=2}^{k} \frac{\partial \pi_{ \theta}(1) }{\partial \theta_j}N_j = \sum_{j=2}^{k} \left( - \sum_{i=2}^{k} \frac{\partial \pi_{ \theta}(i) }{\partial \theta_j}N_j \right) =   \sum_{i=2}^{k}\left( - \sum_{j=2}^{k} \frac{\partial \pi_{ \theta}(i) }{\partial \theta_j}N_j \right) = -\sum_{i=2}^{k} D_i = D_1,
\]
where the first equality uses that $\pi_{\theta}(1)+\cdots+\pi_{ \theta}(k)=1$ and the final equality uses that $D_1 + \cdots + D_k = 0$ for any feasible descent direction.
