# Supplementary material for: Global Optimality Guarantees For Policy Gradient Methods
Source: arXiv:1906.01786 source file (2022-06-20)
Supplement: Supplementary file 2 [file appendix_rates_old.tex]

%!TEX root = policy_grad_optimality.tex

\section{Background: First order methods.}
Throughout we consider the problem of minimizing a smooth function $f: \X \to \mathbb{R}$ over a non-empty, compact and convex set, $\D$
\[
\min_{x \in \D} \, f(x)
\]
A standard defintion of smoothness is stated below. Smoothness also implies a \textit{descent lemma} which will be useful in proving our results throughout.
\begin{definition}[$L$-smoothness]
	\label{def:smoothness}
	A function $f:\mathcal{X}\to \mathbb{R}$ is $L$-smooth over a set $\mathcal{D} \subseteq \X$ if it is differentiable over $\mathcal{D}$ and satisfies,
	\[
	\norm{\nabla f(x) - \nabla f(y)}_2 \leq L \norm{x - y}_2 \,\,\,\, \forall \, x,y \in \mathcal{D}
	\]
	where $L > 0$ is called the smoothness parameter. 
\end{definition}

\begin{lem}[Descent Lemma] \label{lemma:smoothness}
	If the function $f:\mathcal{X}\to \mathbb{R}$ is $L$-smooth over a set $\mathcal{D} \subseteq \X$, then for any $x,y \in \mathcal{D}$:
	\[
	f(y) \leq f(x) + \langle \nabla f(x), y-x \rangle + \frac{L}{2} \norm{y-x}^2_2.
	\]
\end{lem}

\subsection{Convergence of first order methods to stationary points for smooth objectives:}\label{appendix:first_order_methods_proof}
We state and prove Lemma \ref{lemma: first_order_smooth_stationary} which shows that first order methods converge to an $\epsilon$-stationary point in $\mathcal{O}(1/\epsilon^2)$ iterations for smooth objectives. Recall that $x$ is defined to be an $\epsilon$-stationary point if:
\[
    \langle \nabla f(x), x'-x \rangle \geq -\epsilon \quad \forall \, x' \in \mathcal{D}
\]
 
\paragraph{Restatement of Lemma \ref{lemma: first_order_smooth_stationary}:}
Assume $f(\cdot)$ to be $L$-smooth. Let $x^* = \argmin_{x \in \D} \, f(x)$ and define $R:= \sup_{x,y \in \D} \, \norm{x-y}_2$. For any initial point, $x_0$, assume either the projected gradient descent is applied with a constant stepsize $\alpha_t = \alpha \leq \frac{1}{L}$ or the Frank-Wolfe algorithm is applied with $\alpha_t = \frac{\epsilon}{LR^2}$. Then, $x_t$ is guaranteed to be an $\epsilon$-stationary point for
\[
t \geq \frac{2LR^2 (f(x_0)-f(x^*))}{\epsilon^2} \quad \forall \, \epsilon \leq L R^2
\]

\begin{proof}[Proof of Lemma \ref{lemma: first_order_smooth_stationary}]
A simple proof idea underlies the proof for both the algorithms. At every step of the algorithm, we show that either the current iterate is an $\epsilon$-stationary point or the update step reduces the objective function by $\mathcal{O}(\epsilon^2)$. Therefore, we are guaranteed to reach an $\epsilon$-stationary point in $\mathcal{O}(\frac{1}{\epsilon^2})$ iterations. \\

\noindent \underline{\textit{Projected gradient descent}}: Recall that the projected gradient updates take the form:
\[
x_{t+1} = \Pi_\D \left( x_t - \alpha_t \nabla f(x_t) \right)
\]
where $\Pi_{D}$ is the projection operator defined as $\Pi_{\D} (x) = \argmin_{y \in \D} \, \norm{y - x}^2_2$. Equivalently, the update step can also be shown as the  minimizer of a quadratic approximation at the current iterate:
\begin{align}\label{eq:quad_approx_appendix}
    x_{t+1} = \argmin_{x \in \D} \left[ f(x_t) + \langle \nabla f(x_t), x-x_t \rangle + \frac{1}{2\alpha_t} \norm{x-x_t}^2_2 \right]
\end{align}
We assume throughout a constant stepsize, $\alpha_t = \alpha \leq \frac{1}{L}$. Using the descent lemma, we have:
\[
f(z) \leq f(x) + \langle \nabla f(x), z-x \rangle + \frac{1}{2 \alpha}    \norm{z-x}^2_2 \qquad \forall \, z \in \D
\]
Assume that iterate $x_t$ is not an $\epsilon$-stationary point. Then, by definition, there exists a $y \in \D$ such that $\langle \nabla f(x_t), y-x_t \rangle < -\epsilon$ which implies that $x_t \to y$ is a feasible descent direction. Note that as any point along the direction $x_t \to y$ can be represented as $x_t + \beta(y-x_t)$ for $\beta \in [0,1]$, optimizing over $\beta$ decrease the function value by:
\[
\min_{\beta \in [0,1]} \, \left[ \langle \nabla f(x_t), x_t + \beta(y-x_t) - x_t \rangle + \frac{1}{2\alpha} \norm{x_t + \beta(y-x_t) - x_t}^2_2 \right]
\]
Simplifying and using \eqref{eq:quad_approx_appendix} above, we get
\begin{align*}
	f(x_{t+1}) - f(x_t) &\leq \min_{x \in \D} \, \left[ \langle \nabla f(x_t), x-x_t \rangle + \frac{1}{2\alpha} \norm{x-x_t}^2_2 \right] \\
	&\leq \min_{\beta \in [0,1]} \, \left[ \beta \langle \nabla f(x_t), (y-x_t) \rangle + \frac{\beta^2}{2\alpha} \norm{y-x_t}^2_2 \right] \\
	&= \min_{\beta \in [0,1]} \, \left[ -\beta \epsilon + \frac{\beta^2 R^2}{2\alpha} \right] = \frac{-\alpha \epsilon^2}{2R^2}
\end{align*}
for all $\epsilon \leq LR^2$. Here, the second inequality clearly holds as optimizing over the descent direction is clearly sub-optimal to searching over the entire feasible set. Thus, if the current iterate, $x_t$, is not an $\epsilon$-stationary point, we can lower bound the progress of a projected gradient update as:
\[
f(x_t)-f(x_{t+1}) \geq \frac{\alpha \epsilon^2}{2R^2}
\]
Therefore, the algorithm is guaranteed to find an $\epsilon$-stationary point for $t \geq \frac{2 R^2 (f(x_0)-f(x^*))}{\alpha \epsilon^2}$ iterations. As $\alpha_t = \alpha \leq \frac{1}{L}$, our desired result follows. \\
	

\noindent \underline{\textit{Frank-Wolfe Algorithm}}: Recall, the Frank-Wolfe updates take the form:
\begin{align*}
y_t &= \argmin_{y \in \D} \, \langle \nabla f(x_t), y-x_t \rangle \\
x_{t+1} &= x_t + \alpha_t (y_t - x_t)
\end{align*}
for all $t \in \{0,1,\ldots\}$ and $\alpha_t \in (0,1]$. As the objective $f(\cdot)$ is assumed to be $L$-smooth, the descent lemma implies
\begin{align}
	f(x_{t+1}) &\leq f(x_t) + \langle \nabla f(x_t), x_{t+1}-x_t \rangle + \frac{L}{2} \norm{x_{t+1}-x_t}^2_2 \nonumber \\
	&= f(x_t) + \alpha \langle \nabla f(x_t), y_t-x_t \rangle + \frac{\alpha^2 L}{2} \norm{y_t-x_t}^2_2 \nonumber \\
	&\leq f(x_t) + \alpha \langle \nabla f(x_t), y_t-x_t \rangle + \frac{\alpha^2 L R^2}{2} \label{eq:cond_descent_appendix}
\end{align}
where we used that $x_{t+1} = x_t + \alpha_t (y_t - x_t)$, step-size $\alpha \in (0,1]$ and $\norm{y_t-x_t}_2 \leq R$ which follows by assumption. Assume that iterate $x_t$ is not an $\epsilon$-stationary point. Then, there exists a $z \in \D$ such that $\langle \nabla f(x_t), z-x_t \rangle < -\epsilon$. Thus, 
\[
\min_{y \in \D} \, \langle \nabla f(x_t), y-x_t \rangle \leq \langle \nabla f(x_t), z-x_t \rangle < -\epsilon
\]
Using this along with \eqref{eq:cond_descent_appendix} implies,
\[
f(x_{t+1}) - f(x_t) \leq \min_{\alpha \in (0,1]} \, \left[ -\alpha \epsilon + \frac{\alpha^2 LR^2}{2} \right] = \frac{- \epsilon^2}{2 LR^2} 
\]
for $\alpha = \frac{\epsilon}{LR^2}$. Thus, if $x_t$ is not a stationary point then we reduce the function value by atleast $\frac{\epsilon^2}{2LR^2}$. The Frank-Wolfe algorithm therefore finds an $\epsilon$-stationary point for $t \geq \frac{2LR^2 (f(x_0)-f(x^*))}{\epsilon^2}$ iterations as desired.
\end{proof}



\subsection{First order methods with gradient dominated and smooth objectives:}\label{appendix:first_order_gradient_dominated}
We state and prove Lemma \ref{lemma: first_order_smooth_stationary} which shows that first order methods converge geometrically for smooth and second order gradient dominated objectives.

\paragraph{Restatement of Lemma \ref{lemma:second_order_convergence_rate}}:
Assume $f(\cdot)$ is $L$-smooth and second order gradient dominated with modulus $c$. Let $x^* = \argmin_{x \in \D} \, f(x)$. For any initial point, $x_0$ and constant step-size $\alpha$ such that $\alpha c < 1$,
\[
f(x_{t+1}) - f(x^*) \leq \left( 1-\alpha c \right)^t \left( f(x_0) - f(x^*) \right)
\]

\begin{proof}[Proof of Lemma \ref{lemma:second_order_convergence_rate}]

A simple idea underlies the proof for both the algorithms. Essentially, at every step of the algorithm, we use the gradient dominance condition to show a lower bound on the progress, $f(x_t)-f(x_{t+1})$, in terms of the optimality gap, $f(x_t)-f(x^*)$ which enables a geometric convergence rate. \\


\noindent \underline{\textit{Projected gradient descent}}: Note that at any iterate $x_t \neq x^*$, the second-order gradient dominance condition implies that:
\[
\min_{y \in \D} \left[ \langle \nabla f(x_t), y - x_t \rangle + \frac{c}{2} \norm{y-x_t}^2_2 \right] \leq f(x^*) - f(x_t) < 0
\]
Therefore, $\min_{y \in \D} \, \langle \nabla f(x_t), y - x_t \rangle < 0$. The convergence rate then follows immediately using a simple argument:
\begin{align}
	f(x^*) - f(x_t) &\geq \min_{y \in \D} \left[ \langle \nabla f(x_t), y - x_t \rangle + \frac{c}{2} \norm{y-x_t}^2_2 \right] \label{eq:second_order_rate_one}\\
	&= \frac{1}{\kappa} \cdot \min_{y \in \D} \left[ \langle \nabla f(x), y - x \rangle + \frac{1}{2 \alpha} \norm{y-x}^2_2 \right] \label{eq:second_order_rate_two}\\
	&\geq \frac{1}{\kappa} \cdot \left( f(x_{t+1}) - f(x_t) \right) \nonumber 
\end{align}
The final inequality follows by interpreting the projected gradient update, $x_{t+1}$, as the minimizer of a quadratic approximation at $x_t$ (see  Equation \eqref{eq:quad_approx_appendix}). Rearranging, we get:
\[
f(x_{t+1}) - f(x^*) \leq \left( 1-\kappa \right) \left( f(x_t) - f(x^*) \right) \leq \left( 1-\kappa \right)^t \left( f(x_0) - f(x^*) \right)
\]
which shows our desired result. We use the following argument in going from Equation  \eqref{eq:second_order_rate_one} to \eqref{eq:second_order_rate_two}. Let $\bar{y} = \argmin_{y \in \D} \, \langle \nabla f(x), y-x \rangle$ and assume that $\langle \nabla f(x), \bar{y}-x \rangle = -\delta$ for some small $\delta > 0$. Then, for any $c > 0$
\begin{align*}
	\min_{y \in \D} \left[ \langle \nabla f(x), y - x \rangle + \frac{c}{2} \norm{y-x}^2_2 \right] &= \min_{\beta \in [0,1]} \left[ \langle \nabla f(x), x + \beta(\bar{y}-x) - x \rangle + \frac{c}{2} \norm{x + \beta(\bar{y}-x) - x}^2_2 \right] \\
	&= \min_{\beta \in [0,1]} \, \left[ \beta \langle \nabla f(x), \bar{y}-x \rangle + \frac{\beta^2 c}{2} \norm{\bar{y}-x}^2_2 \right] \\
	&= \min_{\beta \in [0,1]} \, \left[ -\beta \delta + \frac{\beta^2 c}{2} \norm{\bar{y}-x}^2_2 \right] \\
	&= \frac{-\delta^2}{2c \norm{\bar{y}-x}^2_2}
\end{align*}
where the first equality follows by arguing that the minimizer of the left had side can be obtained by optimizing along the steepest descent direction, $x_t \to \bar{y}$. This clearly implies that for any $\alpha > 0$,
\[
\min_{y \in \D} \left[ \langle \nabla f(x), y - x \rangle + \frac{c}{2} \norm{y-x}^2_2 \right] = \frac{1}{\kappa} \cdot \min_{y \in \D} \left[ \langle \nabla f(x), y - x \rangle + \frac{1}{2 \alpha} \norm{y-x}^2_2 \right]
\]
where $\kappa = \alpha c$.
\end{proof}
